# Supplementary material for: Statistical transmutation in doped quantum dimer models
Source: arXiv:1202.3618 source file (2012-07-09)
Supplement: Supplementary file 1 [file supplemental_material.pdf]

# Supplemental material for "Statistical transmutation in doped quantum dimer models".


C.A. Lamas,[1] A. Ralko,[2] D.C. Cabra,[3] D. Poilblanc,[1] and P. Pujol[1]

[1]*Laboratoire de Physique Théorique, IRSAMC, CNRS and Université de Toulouse, UPS, F-31062 Toulouse, France*
[2]*Institut Néel, CNRS and Université Joseph Fourier, F-38042 Grenoble, France*
[3]*IFLP, Departamento de Física, Universidad Nacional de La Plata, La Plata, Argentina.*



In this supplementary material, we present further details on the derivation of the proof for statistical transmutation of holons and more technical details regarding the numerical calculations presented in the paper.


## I. STATISTICAL TRANSMUTATION.

### A. Square lattice

The quantum hard-core dimer model with holons on the two-dimensional square lattice can be represented by the following Hamiltonian:

$$H = H_J + H_V + H_t, \tag{1}$$

with

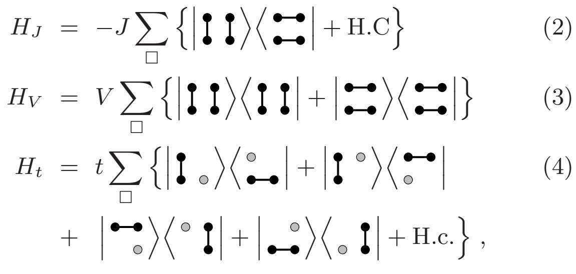

where the sum is over all the elementary plaquettes on the square lattice. Hamiltonian (2) represents the kinetic energy of the dimers and describes the resonance between the two different dimerizations in a square plaquette. The diagonal term (3) is the potential energy. Finally, when dimers change their positions by quantum fluctuations, the holons can move on the lattice across the diagonals of the plaquettes in the square lattice and the term (4) describes the hoping of the holons.

It is convenient to write the Hamiltonian in a second quantized form, by introducing creation operators $b^{\dagger}_{i,j}$ for a dimer sitting between sites $i$ and $j$ and operators $a^{\dagger}_k$ for a hole in the site $k$. In our conventions, dimer configurations are represented by spatially symmetric dimer operators $b^{\dagger}_{i,j}$ that satisfies:

$$\begin{aligned} \left[b_{i,j}, b^{\dagger}_{k,l}\right] &= \delta_{i,k}\delta_{j,l} + \delta_{i,l}\delta_{j,k} \\ \left[b_{i,j}, b_{k,l}\right] &= \left[b^{\dagger}_{i,j}, b^{\dagger}_{k,l}\right] = 0. \end{aligned} \tag{5}$$

This relation reflects the bosonic statistics of the dimers and takes into account its symmetry $b_{i,j} \equiv b_{j,i}$. We introduce the boson operator $a^{\dagger}_i$ which creates a hole in the site $i$ and satisfies

$$\begin{aligned} \left[a_i, a^{\dagger}_j\right] &= \delta_{i,j} \\ \left[a_i, a_j\right] &= \left[a^{\dagger}_i, a^{\dagger}_j\right] = 0, \end{aligned} \tag{6}$$

both operators have bosonic statistics and commutes w.r.t. each other

$$[a_i, b_j] = \left[a^{\dagger}_i, b^{\dagger}_j\right] = \left[a^{\dagger}_i, b_j\right] = 0. \tag{7}$$

Because on each site we are allowed to introduce only one hole or one dimer between the site and one of its nearest neighbors, we introduce the following local constraint:

$$a^{\dagger}_i a_i + \sum_z b^{\dagger}_{i,i+z} b_{i,i+z} = 1. \tag{8}$$

Eq. (8) is independent of the lattice, the sum in $z$ is over all the vectors connecting the site $i$ and its nearest neighbors. In the case of the square lattice, we have $z = \pm\hat{e}_1, \pm\hat{e}_2$ where the vectors $\hat{e}_1$ and $\hat{e}_2$ are the primitive vectors of the direct lattice. Now, in order to change the statistics of the holon operators we apply a 2-D Jordan Wigner transformation on the holon operators[1–4]

$$a_i = e^{-i\phi_i} f_i \tag{9}$$

with

$$\phi_i = \sum_{j\neq i} f^{\dagger}_j f_j \arg(\vec{\tau}_j - \vec{\tau}_i) \tag{10}$$

where $\vec{\tau}_j = x_j + iy_j$, is the complex coordinate of the j-th hole[1]. Notice that there is a freedom in choosing the arguments in (10)[4]. For instance we can arbitrarily shift $\arg(\vec{\tau}_j - \vec{\tau}_i) \to \arg(\vec{\tau}_j - \vec{\tau}_i) + 2n\pi$ with different integer values of $n$ for different pair of sites. This freedom has no physical consequences and we restrict the arguments to the interval $-\pi < \arg(\vec{\tau}_j - \vec{\tau}_i) \leq \pi$. Using that $\arg(\vec{\tau}_i - \vec{\tau}_j) = \arg(\vec{\tau}_j - \vec{\tau}_i) \pm \pi$ and the relations (6) it follows immediately that $f$-operators in different sites anticommutes.

We can calculate the commutation relations between the phase $\phi_i$, written in terms of fermions and $f_j$,

$$\begin{aligned} \phi_i f_j &= \sum_{k\neq i} f^{\dagger}_k f_k f_j \arg(\vec{\tau}_k - \vec{\tau}_i) \\ \phi_i f_j &= f_j(\phi_i - \arg(\vec{\tau}_j - \vec{\tau}_i)) \end{aligned}$$

Then we can write

$$e^{i\phi_i} f_j = f_j e^{i(\phi_i - \arg(\vec{\tau}_j - \vec{\tau}_i))}$$

In a similar way we can show the following relations

$$\begin{aligned} e^{i\phi_i} f_j &= f_j e^{i\phi_i} e^{-i\arg(\vec{\tau}_j - \vec{\tau}_i))} & (11)\\ e^{-i\phi_i} f_j &= f_j e^{-i\phi_i} e^{i\arg(\vec{\tau}_j - \vec{\tau}_i))} & (12)\\ e^{i\phi_i} f_j^\dagger &= f_j^\dagger e^{i\phi_i} e^{i\arg(\vec{\tau}_j - \vec{\tau}_i))} & (13)\\ e^{-i\phi_i} f_j^\dagger &= f_j^\dagger e^{-i\phi_i} e^{-i\arg(\vec{\tau}_j - \vec{\tau}_i))} & (14)\end{aligned}$$

Since in the same site we have $f_i^\dagger f_i = a_i^\dagger a_i$, the constraint (8) and the phase (10) can be written equally in terms of operators $f_i$ or $a_i$:

$$a_i^\dagger a_i + \sum_z b_{i,i+z}^\dagger b_{i,i+z} = f_i^\dagger f_i + \sum_z b_{i,i+z}^\dagger b_{i,i+z} = 1$$

$$\phi_i = \sum_{j\neq i} f_j^\dagger f_j \arg(\vec{\tau}_j - \vec{\tau}_i) = \sum_{j\neq i} a_j^\dagger a_j \arg(\vec{\tau}_j - \vec{\tau}_i).$$

In order to understand the consequences of transformation (9) in the Hamiltonian, the hoping of holons can be written in a general way, independently of the lattice, as a sum of three-site Hamiltonians

$$H_t = \sum h_{(ijk)}^{(t)} \tag{15}$$

with

$$h_{(ijk)}^{(t)} = t\, \hat{\mathcal{P}}\, b_{i,j}^\dagger b_{j,k} a_k^\dagger a_i\, \hat{\mathcal{P}}\,, \tag{16}$$

where we have projected the Hamiltonian on the subspace where the constraint (8) is satisfied by means of the projectors $\hat{\mathcal{P}}$. Making use of the transformation (9) we obtain

$$h_{(ijk)}^{(t)} = t\, e^{i\arg(\vec{\tau}_k - \vec{\tau}_i)} \hat{\mathcal{P}} e^{i\phi_k} e^{-i\phi_i}\; b_{i,j}^\dagger b_{j,k} f_k^\dagger f_i\; \hat{\mathcal{P}}.$$

In the last equation we have changed the boson operators $a_i$ by fermionic ones $f_i$ at the cost of introduce non local interactions. In other words, we have written a boson as a composite particle consisting of an electron with an attached flux.

In order to define new bond operators including the phase $\phi$ in its definition, we must be able to write the phase $\phi$ in terms of operators $b_{i,j}$. This can be performed in the following way: Within the subspace defined by the projector $\hat{\mathcal{P}}$, one can change $\phi$ by $\tilde{\phi}$ in the exponentials, where

$$\tilde{\phi}_i = \sum_{r\neq i} \left[1 - \sum_z b_{r,r+z}^\dagger b_{r,r+z}\right] \arg(\vec{\tau}_r - \vec{\tau}_i)\,, \tag{17}$$

and it is a simple matter to see that

$$\begin{aligned} e^{i\tilde{\phi}_i} b_{j,k} &= b_{j,k} e^{i\tilde{\phi}_i} e^{i[\arg(\vec{\tau}_j - \vec{\tau}_i) + \arg(\vec{\tau}_k - \vec{\tau}_i)]} & (18)\\ e^{-i\tilde{\phi}_i} b_{j,k} &= b_{j,k} e^{-i\tilde{\phi}_i} e^{-i\nu[\arg(\vec{\tau}_j - \vec{\tau}_i) + \arg(\vec{\tau}_k - \vec{\tau}_i)]} & (19)\\ e^{i\tilde{\phi}_i} b_{j,k}^\dagger &= b_{j,k}^\dagger e^{i\tilde{\phi}_i} e^{-i[\arg(\vec{\tau}_j - \vec{\tau}_i) + \arg(\vec{\tau}_k - \vec{\tau}_i)]} & (20)\\ e^{-i\tilde{\phi}_i} b_{j,k}^\dagger &= b_{j,k}^\dagger e^{-i\tilde{\phi}_i} e^{i[\arg(\vec{\tau}_j - \vec{\tau}_i) + \arg(\vec{\tau}_k - \vec{\tau}_i)]} & (21)\end{aligned}$$

Then, using the above relations, we obtain

$$h_{(ijk)}^{(t)} = t e^{i[\pi + \arg(\vec{\tau}_j - \vec{\tau}_i) - \arg(\vec{\tau}_j - \vec{\tau}_k)]} \hat{\mathcal{P}}\; b_{i,j}^\dagger e^{-i\tilde{\phi}_i} e^{i\tilde{\phi}_k} b_{j,k} f_k^\dagger f_i\; \hat{\mathcal{P}}.$$

Now, we attach the flux to dimer operators defining

$$\begin{aligned} \tilde{b}_{i,j}^\dagger &= b_{i,j}^\dagger\, e^{-i(\tilde{\phi}_i + \tilde{\phi}_j)} & (22)\\ \tilde{b}_{i,j} &= e^{i(\tilde{\phi}_i + \tilde{\phi}_j)}\, b_{i,j} & (23)\end{aligned}$$

which allows to write

$$h_{(i,j,k)}^{(t)} = t e^{i[\pi + \arg(\tau_j - \tau_i) - \arg(\tau_j - \tau_k)]} \hat{\mathcal{P}} \tilde{b}_{i,j}^\dagger \tilde{b}_{j,k} f_k^\dagger f_i \hat{\mathcal{P}}. \tag{24}$$

A trivial verification shows that operators $\tilde{b}_{i,j}$ satisfy also to the usual bosonic commutation relations

$$\begin{aligned} \left[\tilde{b}_{i,j}, \tilde{b}_{k,l}\right] &= 0 & (25)\\ \left[\tilde{b}_{i,j}, \tilde{b}_{k,l}^\dagger\right] &= \delta_{i,k}\delta_{j,l} + \delta_{i,l}\delta_{j,k}. & (26)\end{aligned}$$

Transformation (9) together with (22) allows to change the statistics of holes in the QDM from bosonic to fermionic (and vice-versa). After this transformation, the hopping constant $t$ is transformed as

$$\tilde{t}_{(ijk)} = t\, e^{i[\pi + \arg(\tau_j - \tau_i) - \arg(\tau_j - \tau_k)]}. \tag{27}$$

It is then straightforward to write the Hamiltonians (2) and (3) in terms of dimer operators

$$H_J = -J \sum_i \left\{ b_{i,i+e_1}^\dagger b_{i+e_2,i+e_1+e_2}^\dagger b_{i,i+e_2} b_{i+e_1,i+e_1+e_2} \right\}$$

$$H_V = V \sum_i \left\{ b_{i,i+e_2}^\dagger b_{i+e_1,i+e_1+e_2}^\dagger b_{i,i+e_2} b_{i+e_1,i+e_1+e_2} \right\}.$$

and using (22) we can easily write the Hamiltonian in terms of the new dimer operators $\tilde{b}_{j,k}$. Using that $\arg(\vec{\tau}_j - \vec{\tau}_i) = \arg(\vec{\tau}_i - \vec{\tau}_j) \pm \pi$ and evaluating the arguments of the NN vectors, that on the square lattice take the values $\arg(\vec{\tau}_j - \vec{\tau}_i) = 0, \pi, \pm\pi/2$ we finally obtain:

$$H_J = -J \sum_i \left\{ \tilde{b}_{i,i+e_1}^\dagger \tilde{b}_{i+e_2,i+e_1+e_2}^\dagger \tilde{b}_{i,i+e_2} \tilde{b}_{i+e_1,i+e_1+e_2} \right\}$$

$$H_V = V \sum_i \left\{ \tilde{b}_{i,i+e_2}^\dagger \tilde{b}_{i+e_1,i+e_1+e_2}^\dagger \tilde{b}_{i,i+e_2} \tilde{b}_{i+e_1,i+e_1+e_2} \right\}.$$

Then, after this series of transformations we can write the Hamiltonian as $H = \tilde{H}_J + \tilde{H}_V + \tilde{H}_t$ with

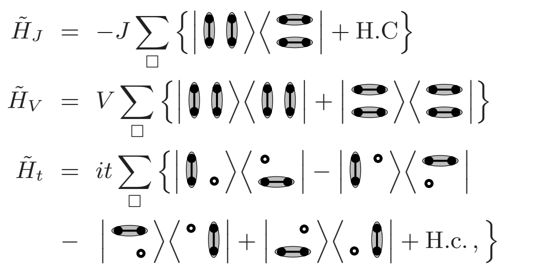

where the dimer and the hole are created by the operators $\tilde{b}^\dagger$ and $f^\dagger$ respectively. Although in the last equation we use a different notation for the dimers, the operators $\tilde{b}^\dagger$ give rise to the same physics than the $b^\dagger$, both are symmetric bosonic operators and satisfy the constraint (8). The kinetic and potential amplitudes for the Hamiltonian corresponding to dimers remain invariant after the J-W transformation, but the amplitude on the holon Hamiltonian is changed. The hoping amplitude becomes imaginary with different sign depending of the direction in holon motion. Although it seems to be a more complicated model, we can use a simple gauge transformation on dimers to eliminate the complex phase $i$ in the hopping Hamiltonian:

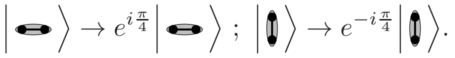

Obtaining

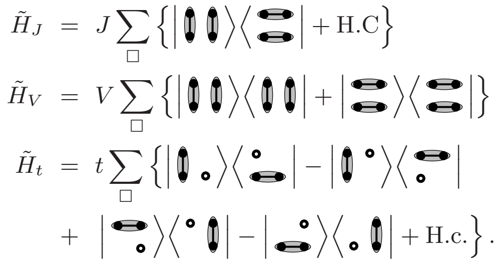

Now, the holon hoping Hamiltonian can be transformed by means of a gauge transformation on the holes, $f_j \to e^{i\vec{Q}\cdot\vec{r}_j} f_j$ with $\vec{Q} = (\frac{\pi}{2}, \frac{\pi}{2})$, to recover the original form in Eq. (1). With this transformation we have that

$$
\begin{aligned}
f^\dagger_{j+e_1+e_2} f_j &\to -f^\dagger_{j+e_1+e_2} f_j \\
f^\dagger_{j+e_1-e_2} f_j &\to f^\dagger_{j+e_1-e_2} f_j ,
\end{aligned}
$$

and finally the Hamiltonian reads $H = \tilde{H}_J + \tilde{H}_V + \tilde{H}_t$ with

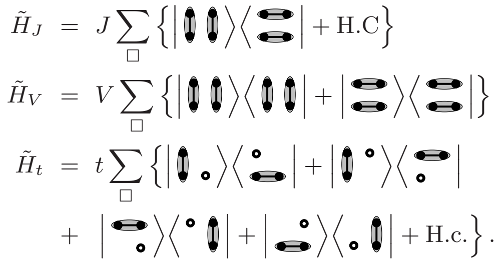

To conclude, choosing a convenient gauge for the dimers and holons we have recovered the original form of the Hamiltonian but with the amplitude for the dimer kinetic term $J$ changed by $-J$. Then, a doped QDM with bosonic holons and flipping constant $J$ is equivalent to the QDM with fermionic holons and $-J$. This equivalence, first discovered on the basis of numerical calculations for the square lattice[5], is here proven exactly.

### B. Triangular lattice

The statistical transmutation symmetry is also valid in non-bipartite lattices and an interesting example is the QDM on the triangular lattice. We shall briefly describe the steps of the proof for the triangular lattice in what follows. We start with a quantum hard-core dimer model with holons on the two-dimensional triangular lattice given by the following Hamiltonian:

$$H = H_{\unicode{x25B1}} + H_{\unicode{x2B54}} + H_{\Diamond} + H^{(t)}_{\triangle} + H^{(t)}_{\triangledown} \tag{28}$$

where

$$H_{\unicode{x25B1}} = H^{(J)}_{\unicode{x25B1}} + H^{(V)}_{\unicode{x25B1}} \tag{29}$$

with

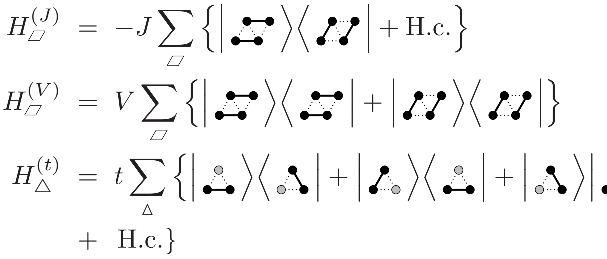

(30)

(31)

(32)

and similar expressions for $H_{\unicode{x2B54}}$, $H_{\Diamond}$ and $H^{(t)}_{\triangledown}$ corresponding to all the orientations of the rhombus and possible hoppings of holons $H_t$ on both up and down orientation of the triangles.

In the triangular lattice the sum in the local constraint (8) is over $z = \pm\hat{r}_1, \pm\hat{r}_2, \pm(\hat{r}_2 - \hat{r}_1)$, with $\hat{r}_1 = (1,0)$ and $\hat{r}_2 = (\frac{1}{2}, \frac{\sqrt{3}}{2})$. The Hamiltonian corresponding to the hopping of holons is projected into the subspace where the constraint is satisfied and can also be written in general as in Eq. (16). Changing the holon operators as in Eq. (9) and dimer operators as in Eq (22) we obtain

$$\tilde{H}_t = te^{i\frac{2}{3}\pi} \sum \hat{\mathcal{P}}\, \tilde{b}^\dagger_{i,j} \tilde{b}_{j,k} a^\dagger_k a_i \,\hat{\mathcal{P}}$$

Now, writing the Hamiltonians $H^{(J)}_{\unicode{x25B1}}$ and $H^{(V)}_{\unicode{x25B1}}$ in terms of the dimer operators $\tilde{b}_{i,j}$ we obtain for the Hamiltonian,

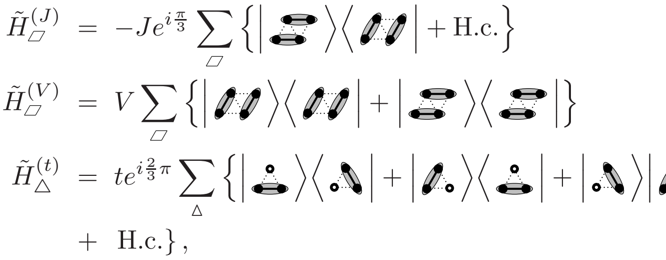

(33)

(34)

(35)

and analogous expressions for the Hamiltonians corresponding to the rotated rhombi. Now, in order to transform the Hamiltonian corresponding to the hopping of holons such that the hopping constant $\tilde{t} = te^{i\frac{2}{3}\pi}$ becomes

real, we use the following gauge transformation on the dimers

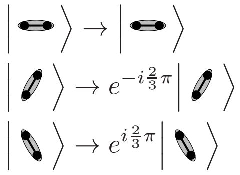


and we finally obtain for the Hamiltonian in terms of fermionic holons and transformed dimers $\tilde{b}_{i,j}$

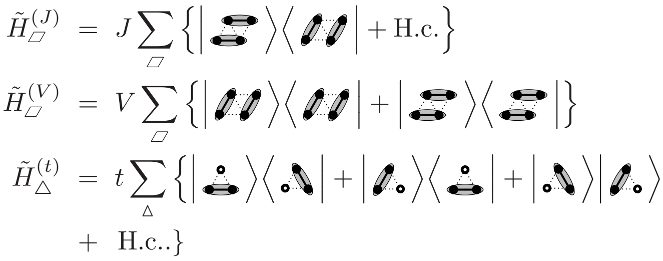


To summarize, as in the square lattice, we obtain the equivalence between, on one hand, the model with fermionic holons and dimer resonance constant $J$ and, on the other hand, the bosonic model with $-J$. We also emphasize that such an equivalence is proven exactly.

## II. PHYSICAL QUANTITIES

### A. Phase separation and the Maxwell construction

At large $J$ compared to the holon average kinetic energy (proportional to $t$) holons tend to separate from the dimer fluctuating background, in order to minimize the dimer resonance energy. The question of *phase separation* (PS), *i.e.* the possibility for the system to spontaneously undergoes a macroscopic segregation into two phases with different hole concentrations, has then to be considered.

Hence, we analyze the GS energy as a function of the holon concentration $x = n_h/N$, where $n_h$ is the number of holons in the system and $N$ the number of sites, for different hopping parameters $t$. In order to perform a Maxwell construction we define:

$$s(x) = \frac{e(x) - e(0)}{x} \tag{36}$$

where $e(x)$ is the energy per site at doping $x$. This quantity is nothing else but the slope of the line passing through $e(0)$ and $e(x)$. In the case of PS, the energy presents a change of curvature at a critical doping $x_c$ corresponding to the minimum of $s(x)$ as a function of $x$. The fact that the local curvature of $e(x)$ at $x = 0$ is negative then implies that the two seperated phases will have $x = x_c$ and $x = 0$ (the undoped insulator) hole concentrations. In Fig. 1 is computed the Maxwell construction for each of the four models considered in our study.

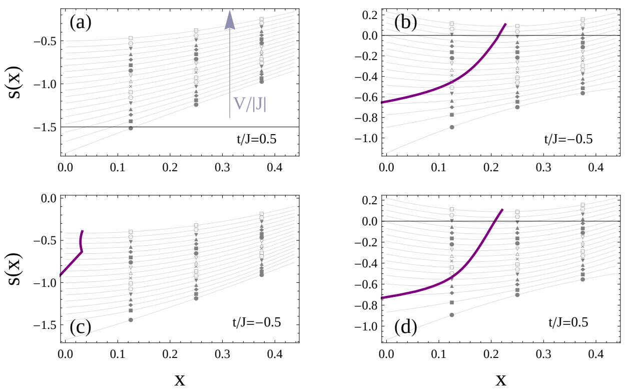


FIG. 1: (color online) Maxwell constructions (grey lines) for the four models considered in our work ((a) to (d)) as a function of the holon density $x$. Thick lines: critical lines $x_c$ corresponding to the minima of the curves used in the construction of the phase diagrams; for (a), (b), (c) and (d), $t/J$ is respectively 0.5, $-0.5$, $-0.5$ and 0.5, and $V/|J|$ is always ranging from 0.0 to 1.0.

### B. The sign operator

Another important quantity used in the paper is the sign operator which provides a quantitative analysis of the nodal structure of the wavefunction and hence gives insights about the statistical nature of the holons, *i.e.* whether they behave as bosons or fermions.

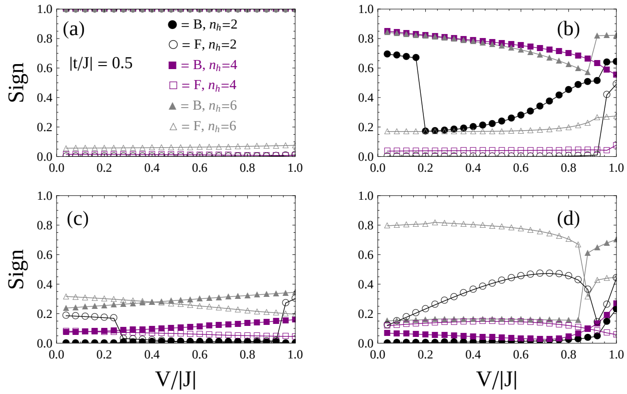


FIG. 2: (color online) Sign operator for the four hamiltonians ((a) to (d)) as a function of V. For each model, we display the $n_h = 2$ (circles), 4 (squares) and 6 (triangles) holons on the 16-site cluster, with both the $R = B$ (filled symbols) and $R = F$ (empty symbols) representations. For (a), (b), (c) and (d), $t/J$ is respectively 0.5, $-0.5$, $-0.5$ and 0.5.

Following Ref. [5] we can make use of the fact that two possible representations of our models are possible, namely either in terms of bosonic or fermionic (bare) operators. It is then convenient to introduce two basis sets of dimer configurations $\{|c_B\rangle\}$ and $\{|c_F\rangle\}$ (labeled ac-

cording to the assumed statistics of the bare holons). These two sets can obviously be transformed into one another by simply changing relative configuration signs within each class $\mathcal{C}$ characterized by some fixed hole positions, as explained in the procedure of Ref. [6]. As mentionned in Ref. [5], this can be physically interpreted as attaching (removing) single vortices next to the holons. Hence, one can define a "fermionic" ($R = F$) and a "bosonic" ($R = B$) average sign as:

$$\mathrm{Sign}_R = \frac{\sum_{\mathcal{C}} \left|\sum_{c\in\mathcal{C}} \langle\psi_0|c_R\rangle \, |\langle\psi_0|c_R\rangle|\right|}{\sum_c |\langle\psi_0|c_R\rangle|^2} \tag{37}$$

where the summations runs over all $\mathcal{C}$ classes and over all dimer configurations within each class. $\mathrm{Sign}_R$ is constructed in such a way that it is maximum and equal to 1 when all GS weights $\langle\psi_0|c_R\rangle$ have the same sign (for fixed hole position), hence characterizing holons of $R$ type. The results of $\mathrm{Sign}_R$ on the 16-site cluster with 2, 4 and 6 holons are depicted for each of the four models in Fig.2.

### C. Flux quantization

Lastly, we investigate flux quantization (to probe the superconducting character of the system) by inserting in the torus an Aharonov-Bohm flux of strength $\phi = \xi\phi_0$ with $0 \leq \xi \leq 1$ and $\phi_0 = hc/e$ the elementary magnetic flux. This is achieved by adding a phase shift in e.g. the x-direction. In other words, one performs the Peierls substitution $t \rightarrow \exp(2i\pi(\xi\vec{u}_x + 2\eta/\sqrt{3}\vec{u}_y)\cdot\vec{u}_i/L)t$ with $\vec{u}_i$ the hopping direction on the triangular lattice of linear size $L$. In addition, arbitrary boundary conditions in the $y$-direction are used to interpolate between the available transverse momenta. Numerical results are shown in the main paper.


[1] Y.R. Wang, Phys. Rev. B **43**, 3786 (1991)
[2] Eduardo Fradkin, Phys. Rev. Lett. **63**, 322 (1989)
[3] C.A. Lamas, A. Ralko, D.C. Cabra, D. Poilblanc and P. Pujol, ArXiv:1202.3618 (2012).
[4] C.A. Lamas, D.C. Cabra, M.D. Grynberg, G.L. Rossini. Phys. Rev. B **74**, 224435 (2006)
[5] D. Poilblanc, Phys. Rev. Lett. **100**, 157206 (2008).
[6] N. Read and B. Chakraborty, Phys. Rev. B 40, 7133 (1989); see also P. Lederer and Y. Takahashi, Z. Phys. B 71, 311 (1988).
[7] Y. Saiga and M. Oshikawa. Phys. Rev. Lett. **96**, 036406 (2006)
[8] A. Ralko, F. Becca and D. Poilblanc, Phys. Rev. Lett. **101**, 117204 (2008);
[9] N. Read and B. Chakraborty, Phys. Rev. B **40**, 7133 (1989)
